# Supplementary material for: A comprehensive study of analyzing powers in the proton-deuteron break-up channel at 135 MeV
Source: arXiv:2006.02268 ancillary file (2020-08-27)
Supplement: Supplementary file 1 [file Supplementary_Material.pdf]

# Supplemental material

belonging to the paper

# A comprehensive study of analyzing powers in the proton-deuteron break-up channel at 135 MeV

M. T. Bayat[1a], H. Tavakoli-Zaniani[1,2], H. R. Amir-Ahmadi[1], A. Deltuva[3], M. Eslami-Kalantari[2], J. Golak[4], N. Kalantar-Nayestanaki[1], St. Kistryn[5], A. Kozela[6], H. Mardanpour[1], J. G. Messchendorp[1b], M. Mohammadi-Dadkan[1,7], A. Ramazani-Moghaddam-Arani[8], R. Ramazani-Sharifabadi[1,9], R. Skibiński[4], E. Stephan[10], and H. Witała[4]

[1] KVI-CART, University of Groningen, Groningen, The Netherlands
[2] Department of Physics, School of Science, Yazd University, Yazd, Iran
[3] Institute of Theoretical Physics and Astronomy, Vilnius University, Saulėtekio al. 3, 10222 Vilnius, Lithuania
[4] M. Smoluchowski Institute of Physics, Jagiellonian University, Kraków, Poland
[5] Institute of Physics, Jagiellonian University, Kraków, Poland
[6] Institute of Nuclear Physics, PAS, Kraków, Poland
[7] Department of Physics, University of Sistan and Baluchestan, Zahedan, Iran
[8] Department of Physics, Faculty of Science, University of Kashan, Kashan, Iran
[9] Department of Physics, University of Tehran, Tehran, Iran
[10] Institute of Physics, University of Silesia, Chorzów, Poland

**Experimental results:** The analyzing powers ($A_x$ and $A_y$) for the chosen configurations are presented in Figs. 1-12. Note that the coplanar configurations $(\theta_1, \theta_2, \phi_{12}) = (107°, 16°, 180°)$, $(107°, 20°, 180°)$ and $(107°, 24°, 180°)$ have been excluded from the analysis, since in those cases, the background from the proton-deuteron elastic channel was overwhelming and could not be reduced significantly by PID. Theoretical predictions, as specified in the legend, show the Faddeev calculations using the 2NF such as CDB [1,2] (dashed-dotted line) and AV18 [3] (dotted line) and 2NF+3NF models such as CDB+$\Delta$ (long-dashed line), CDB+TM99 [4–6] (short-dashed line), AV18+UIX [7] (solid line) and CDB+$\Delta$+Coulomb [8,9] (dashed-double-dotted line).

[a] m.t.bayat@rug.nl
[b] j.g.messchendorp@rug.nl

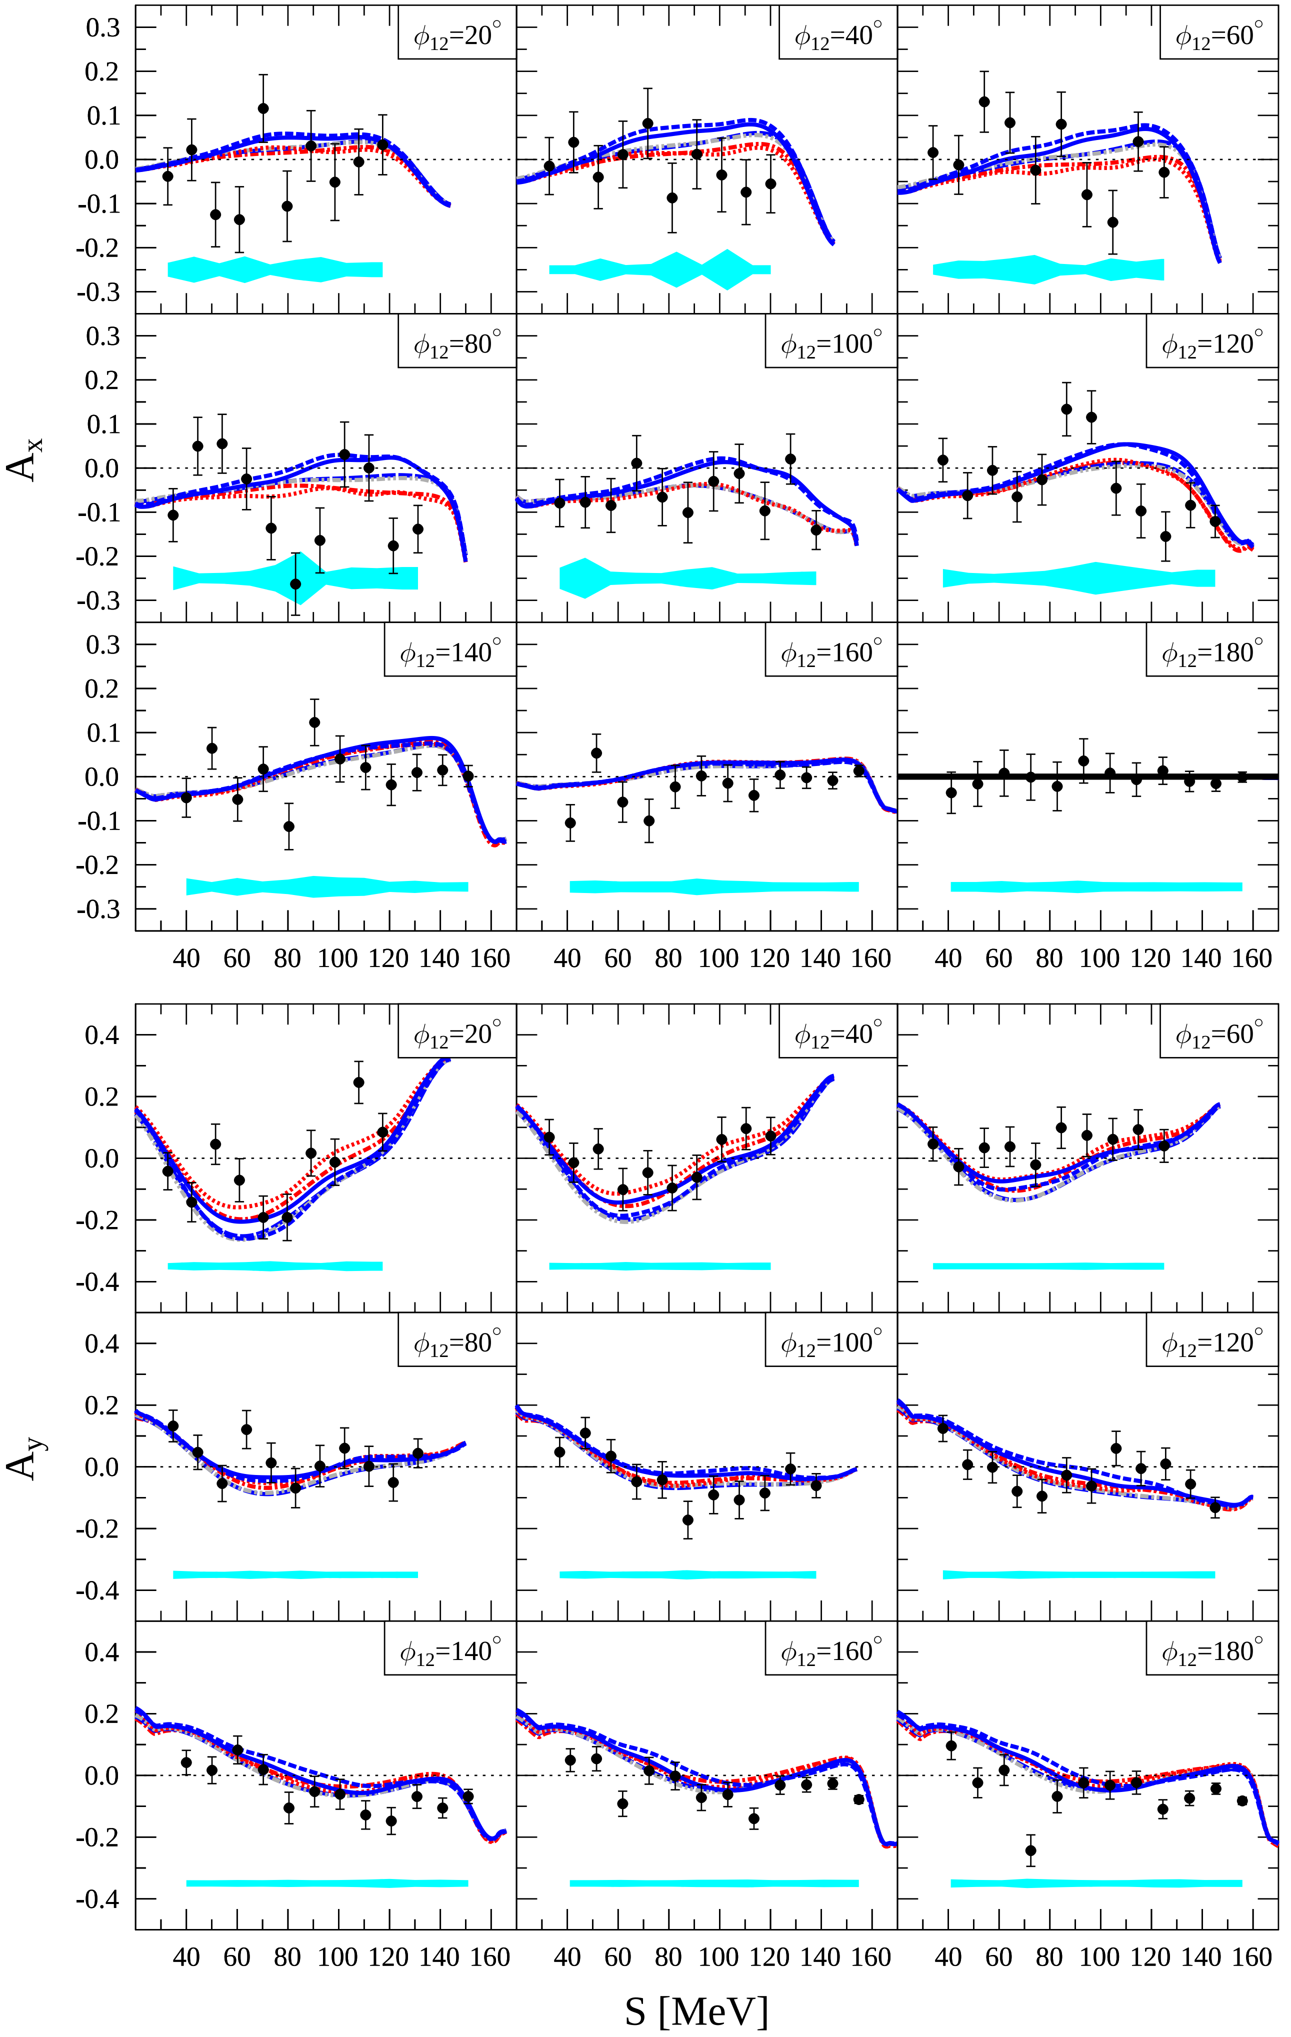


**Fig. 1.** The analyzing powers at ($\theta_1 = 45^\circ, \theta_2 = 16^\circ$) as a function of $S$ for different azimuthal opening angles. Error bars shown reflect only statistical uncertainties. The errors are statistical and the cyan bands depict $2\sigma$ systematic uncertainties.

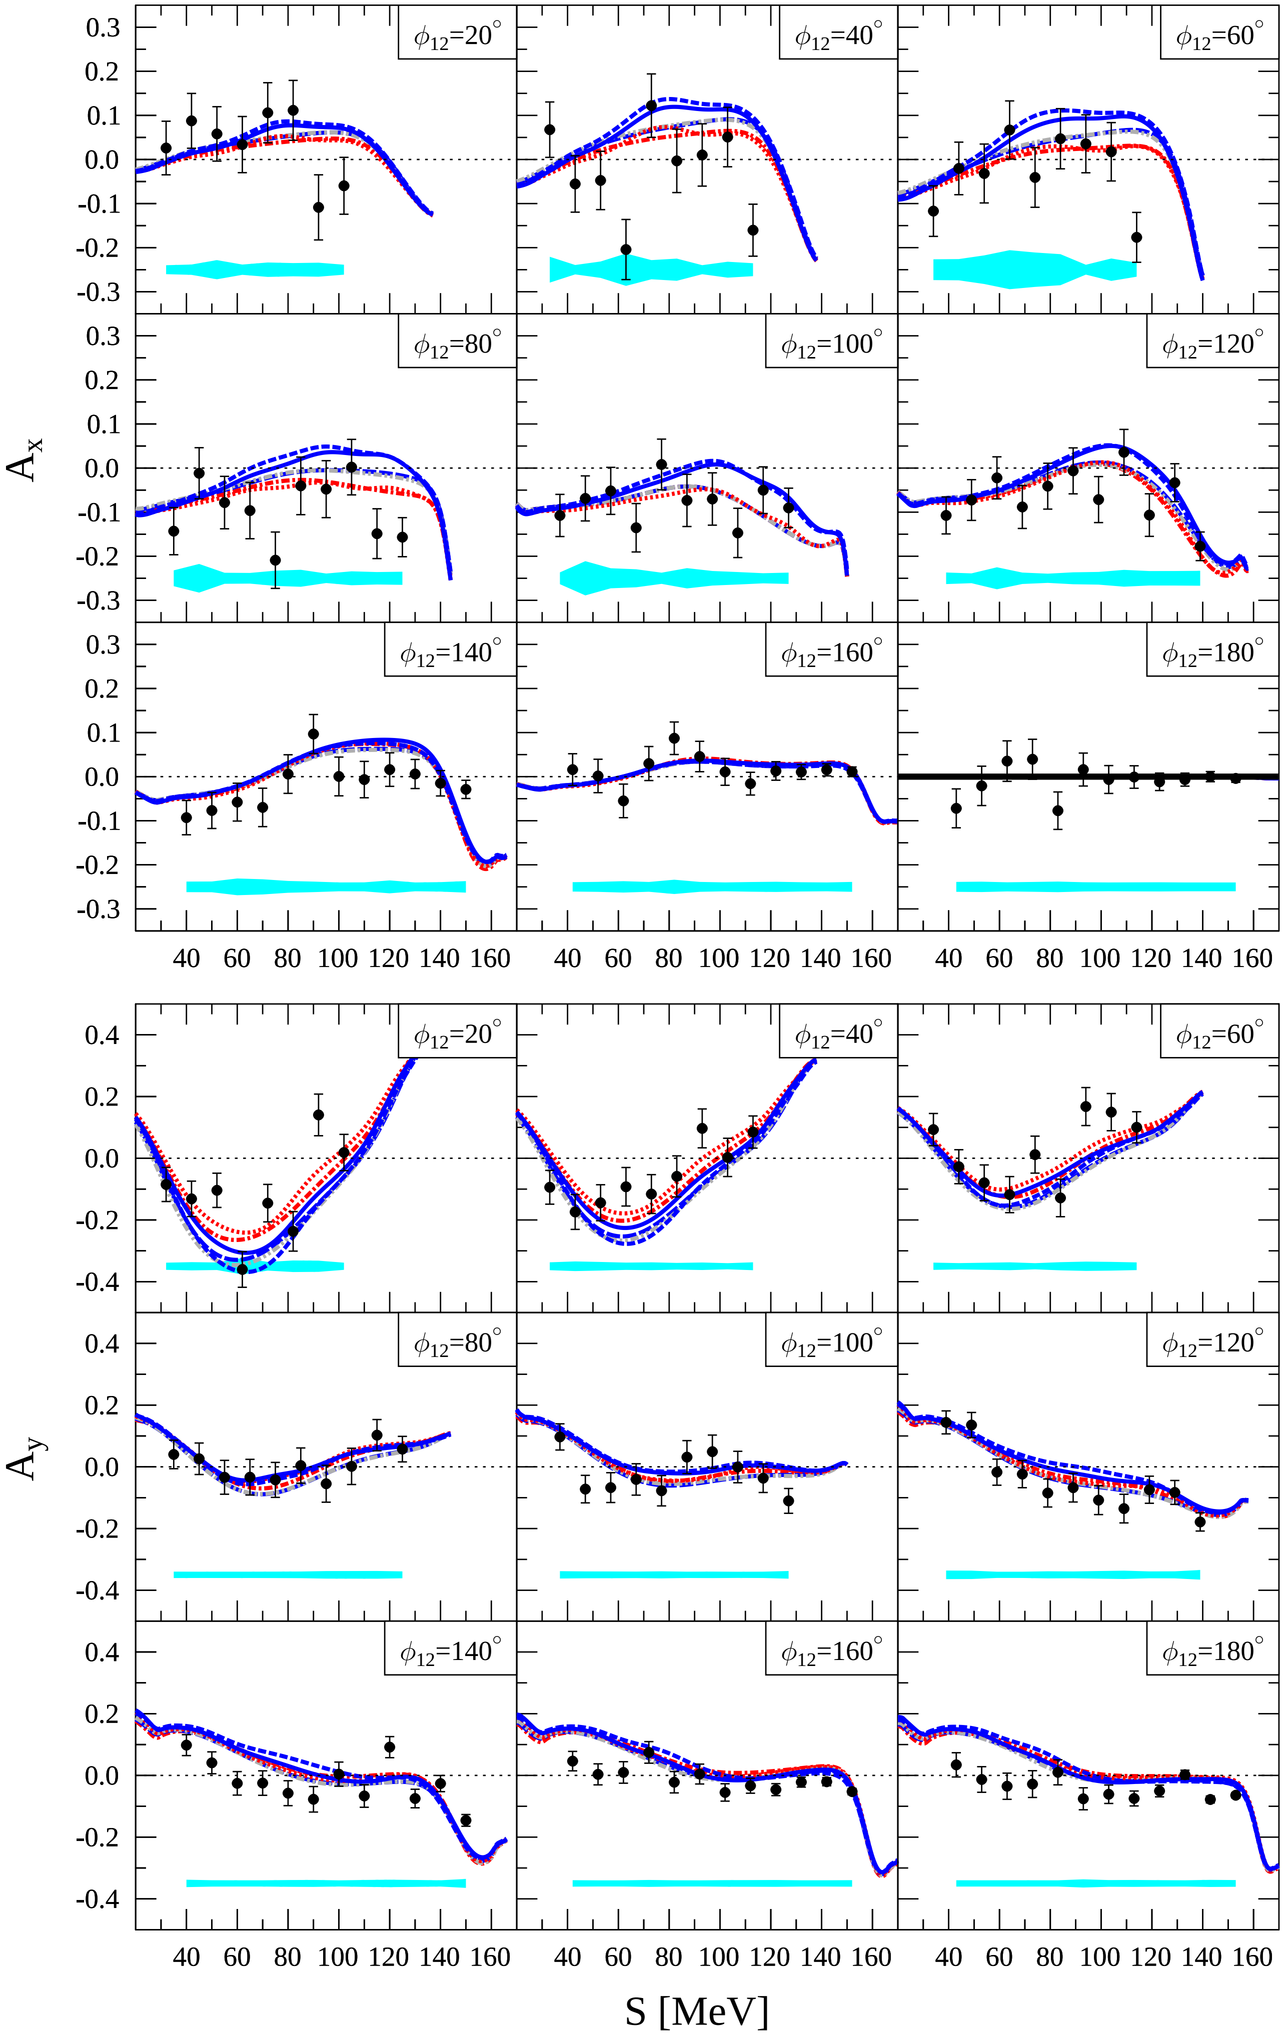


**Fig. 2.** Same as Fig. 1 except for $(\theta_1 = 45^\circ, \theta_2 = 20^\circ)$.

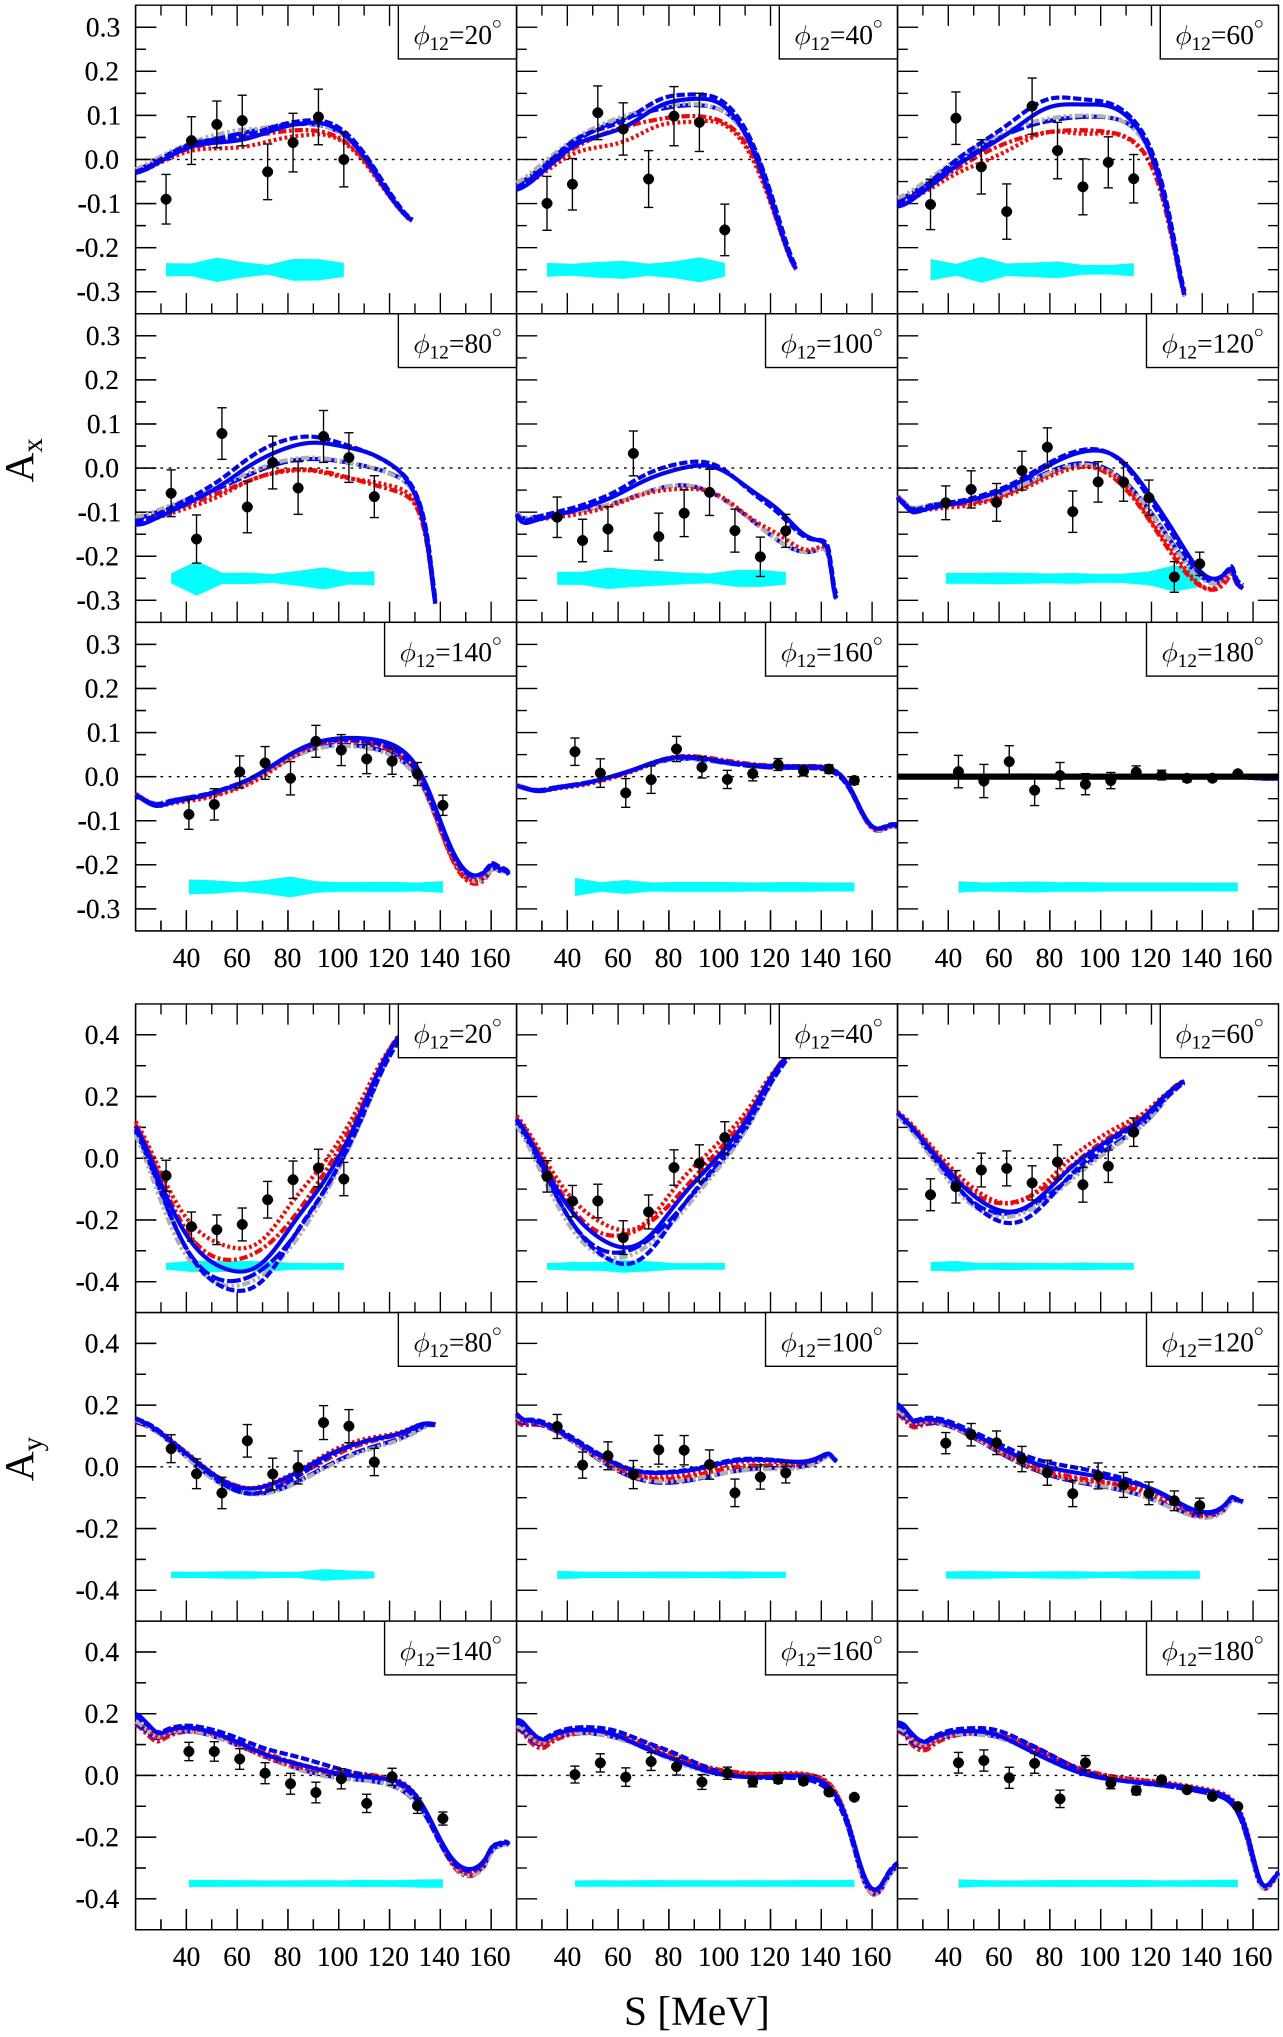


**Fig. 3.** Same as Fig. 1 except for ($\theta_1 = 45°, \theta_2 = 24°$).

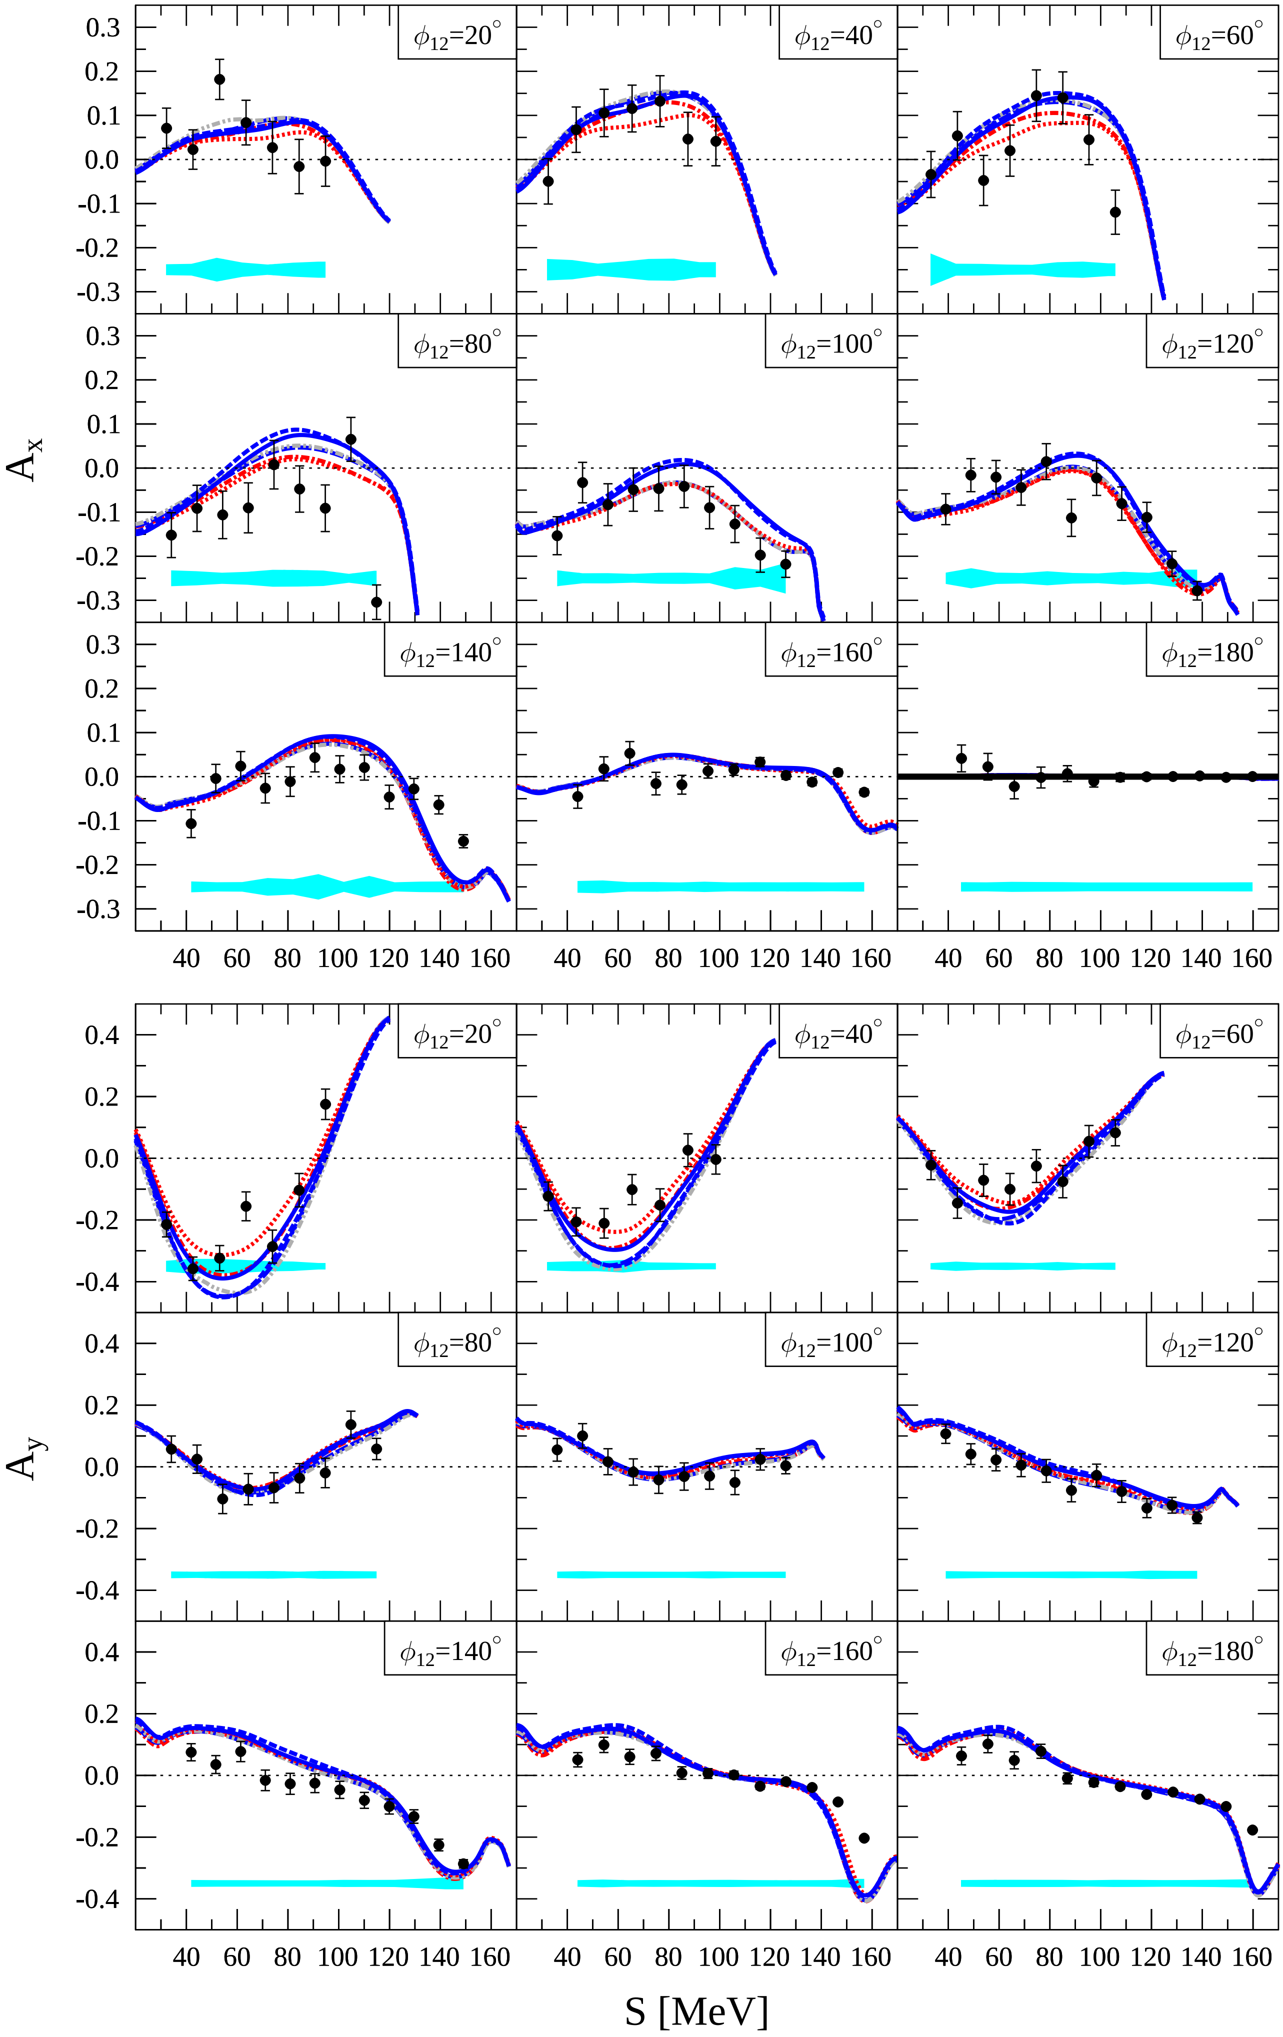


**Fig. 4.** Same as Fig. 1 except for ($\theta_1 = 45^\circ, \theta_2 = 28^\circ$).

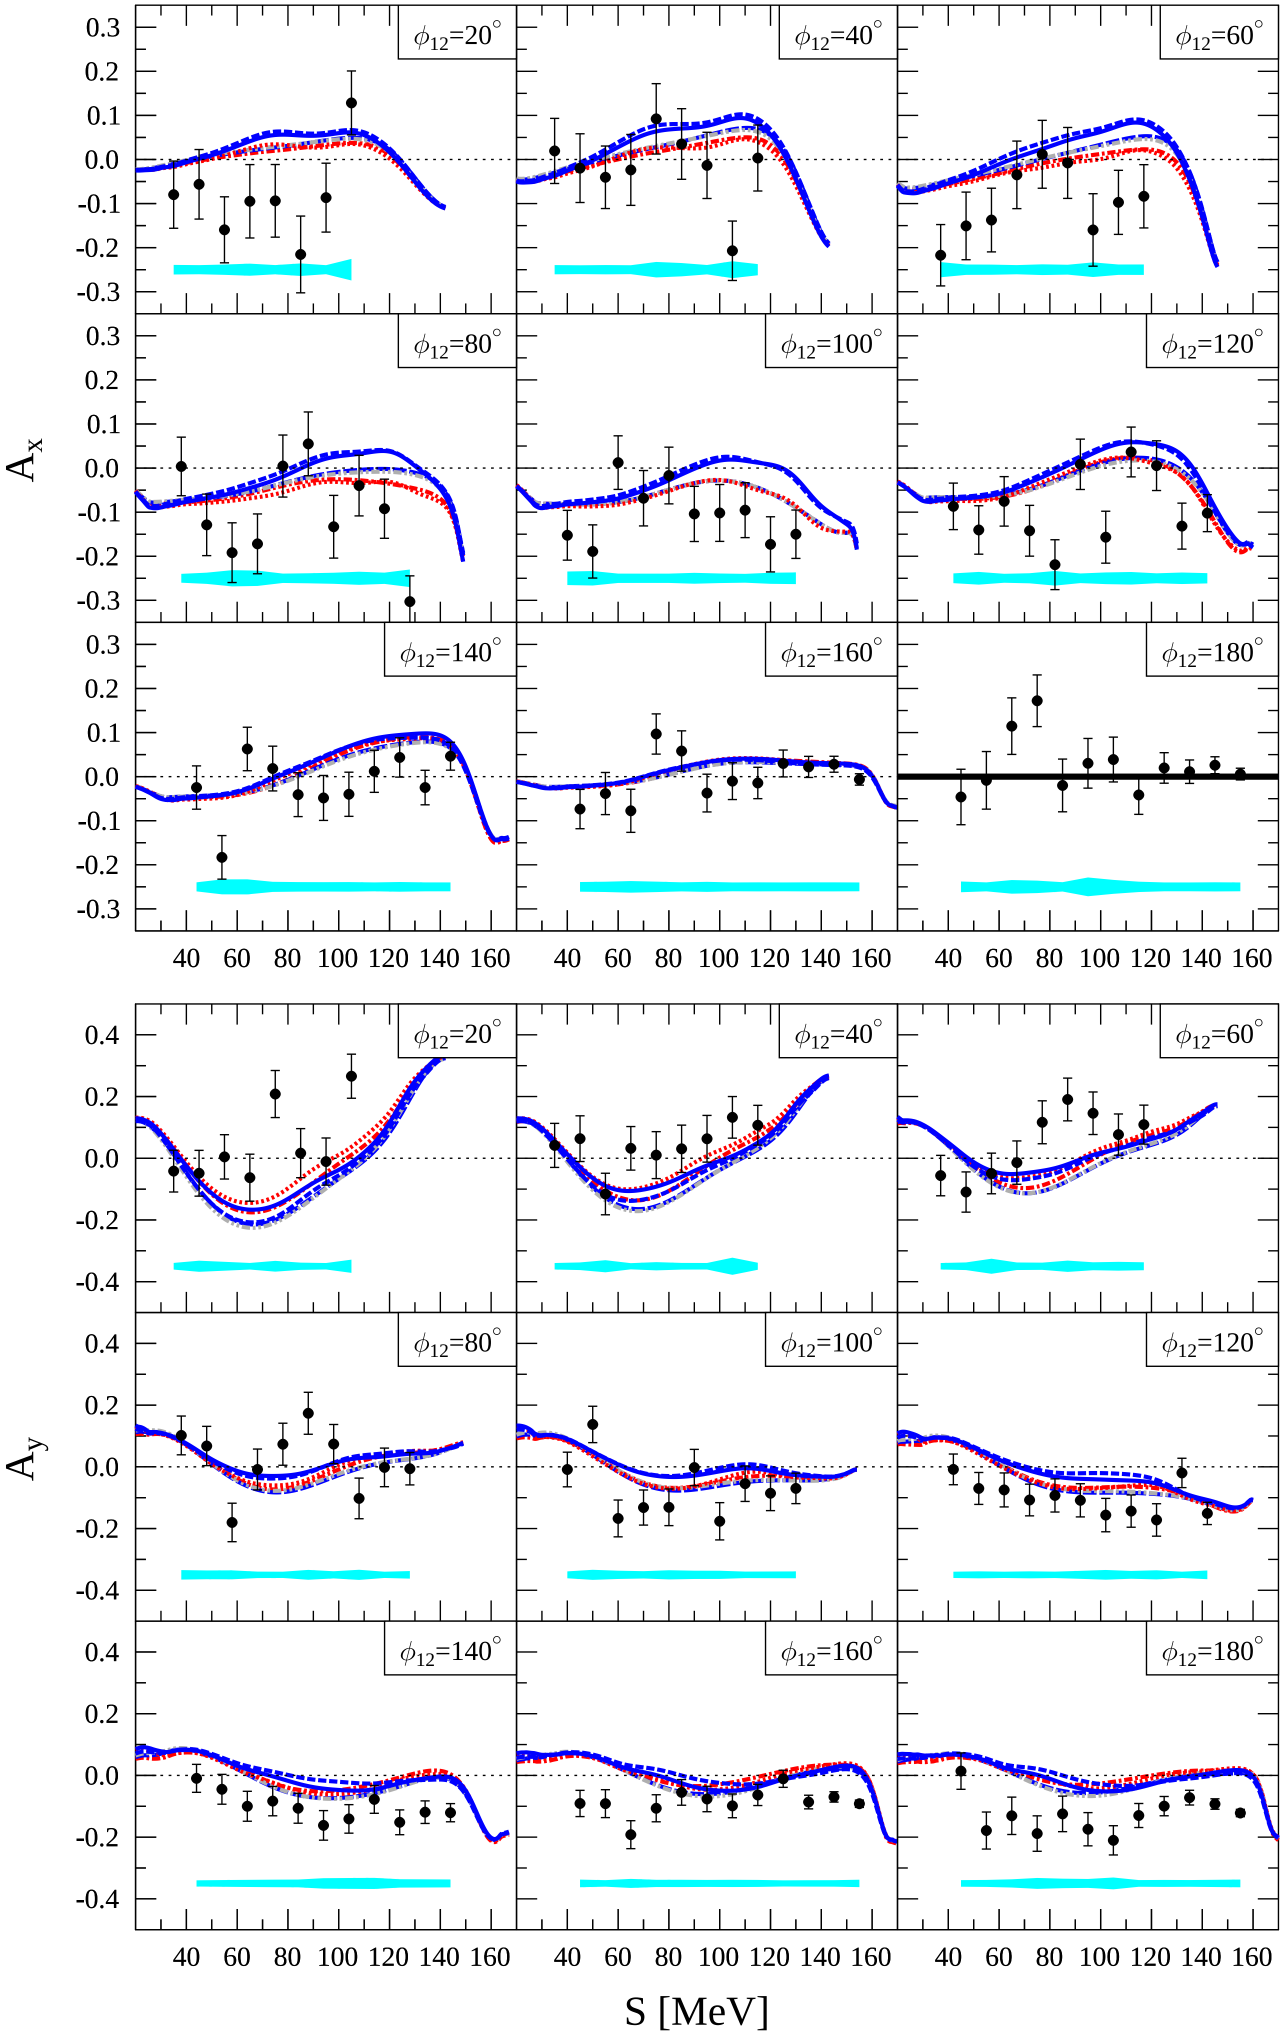


**Fig. 5.** Same as Fig. 1 except for ($\theta_1 = 50°, \theta_2 = 16°$).

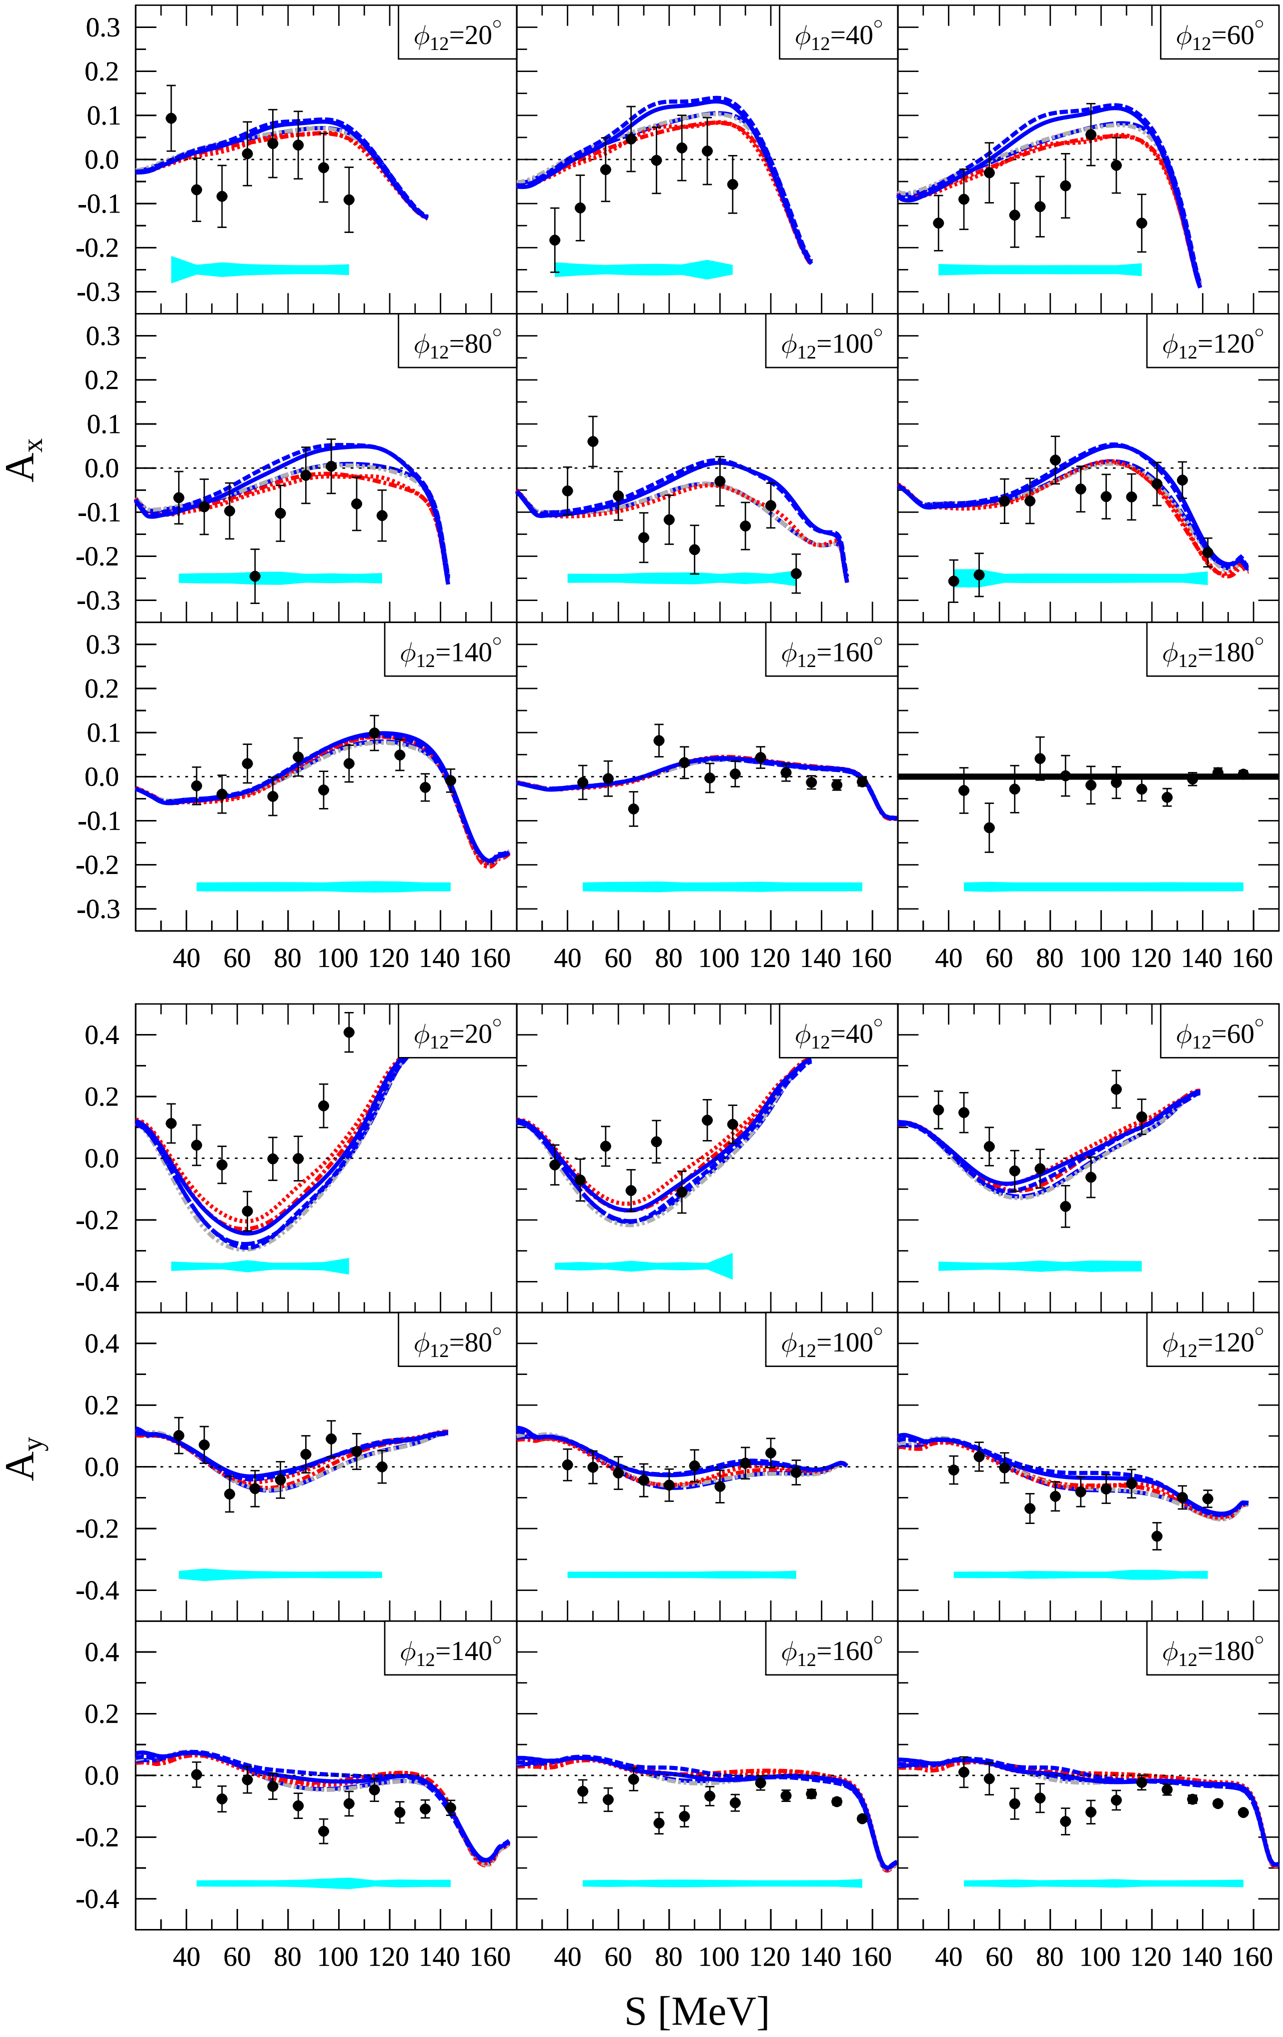


**Fig. 6.** Same as Fig. 1 except for ($\theta_1 = 50°, \theta_2 = 20°$).

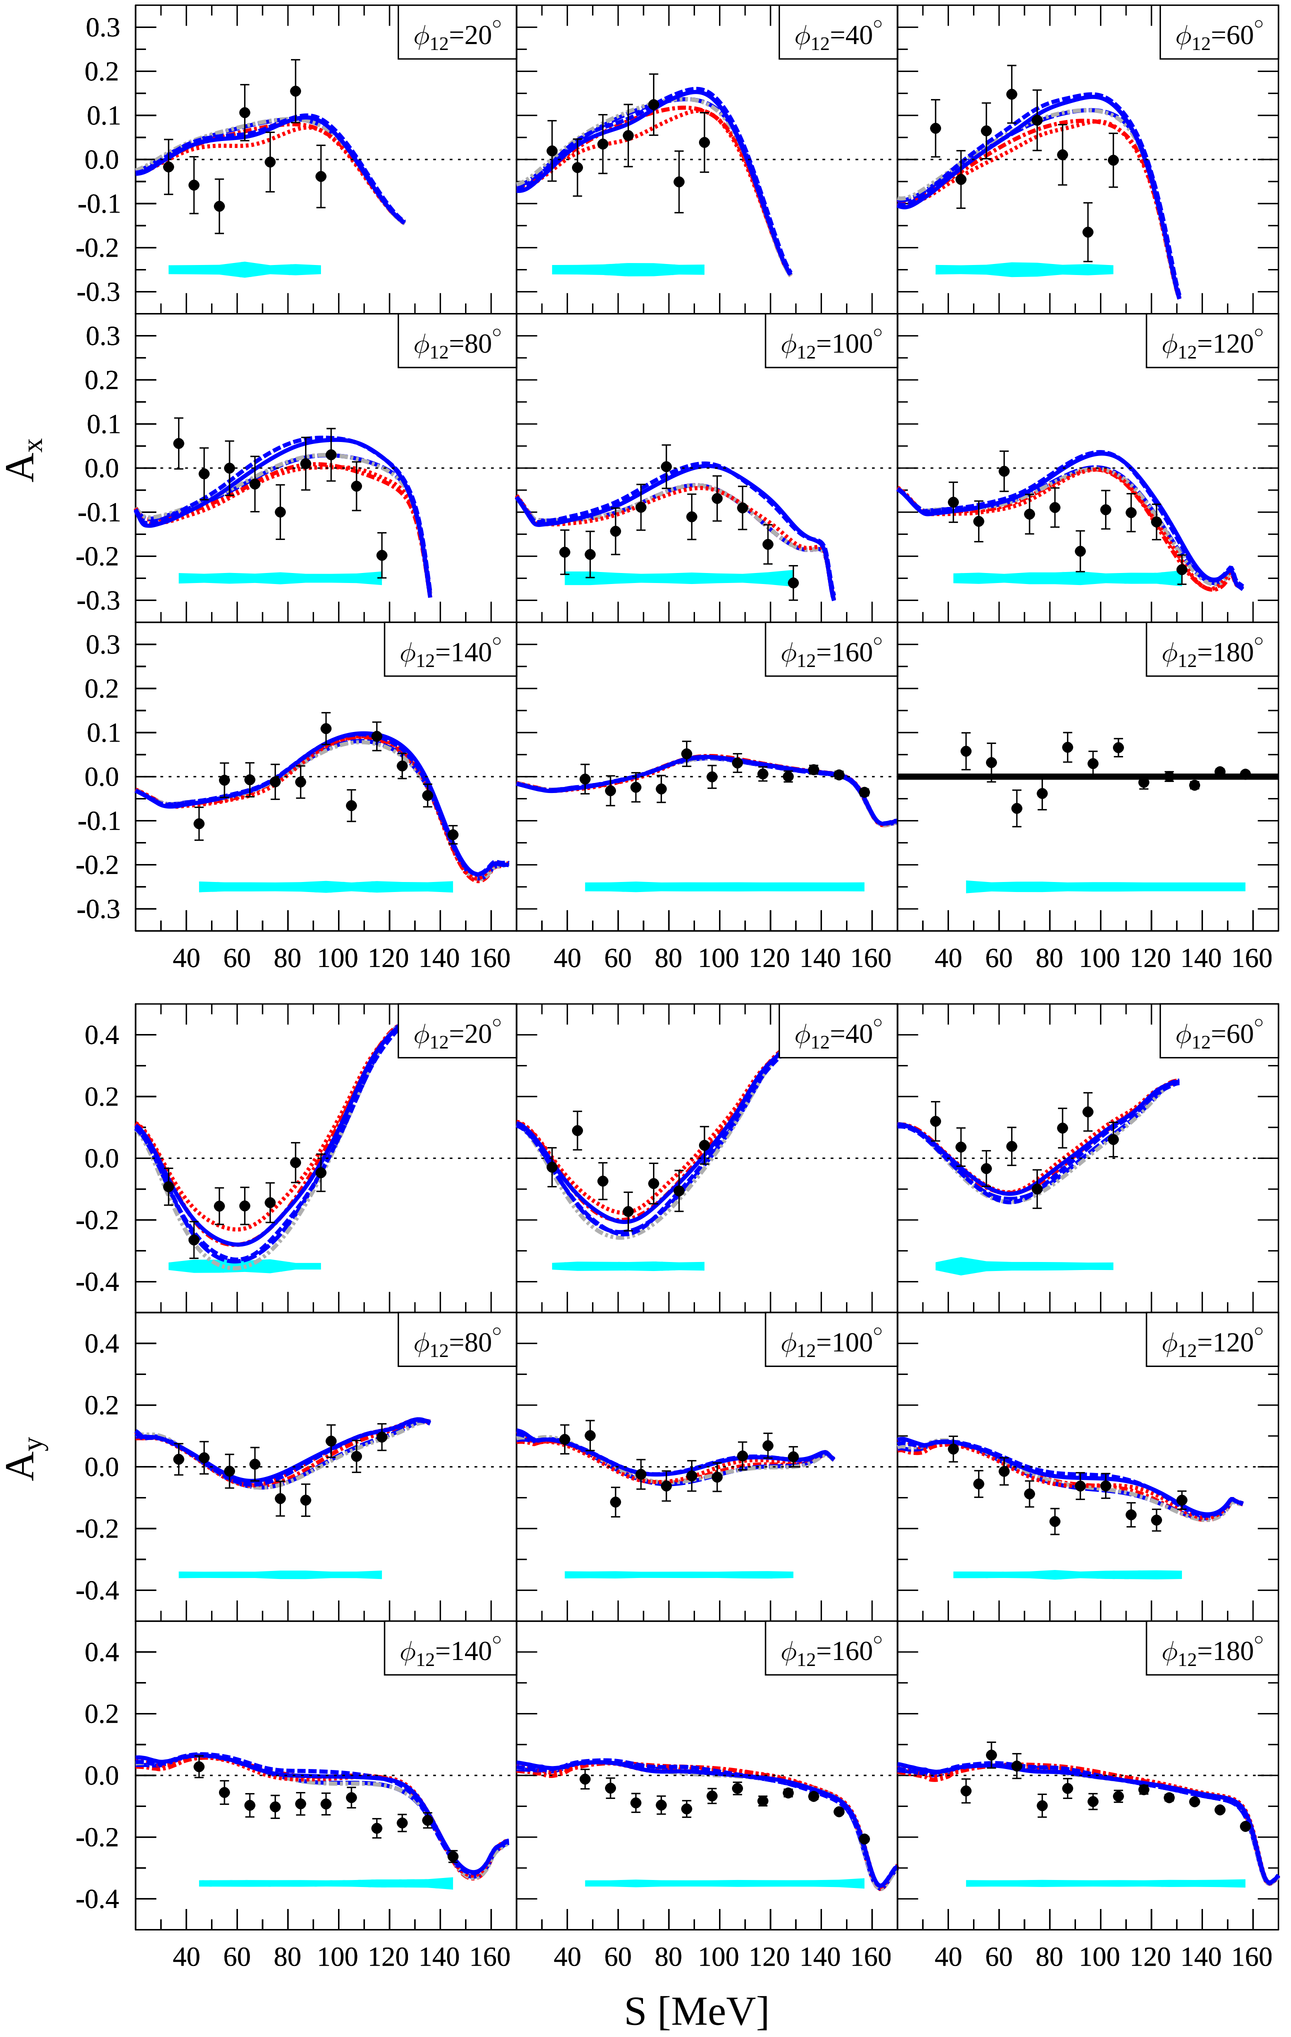


**Fig. 7.** Same as Fig. 1 except for ($\theta_1 = 50^\circ, \theta_2 = 24^\circ$).

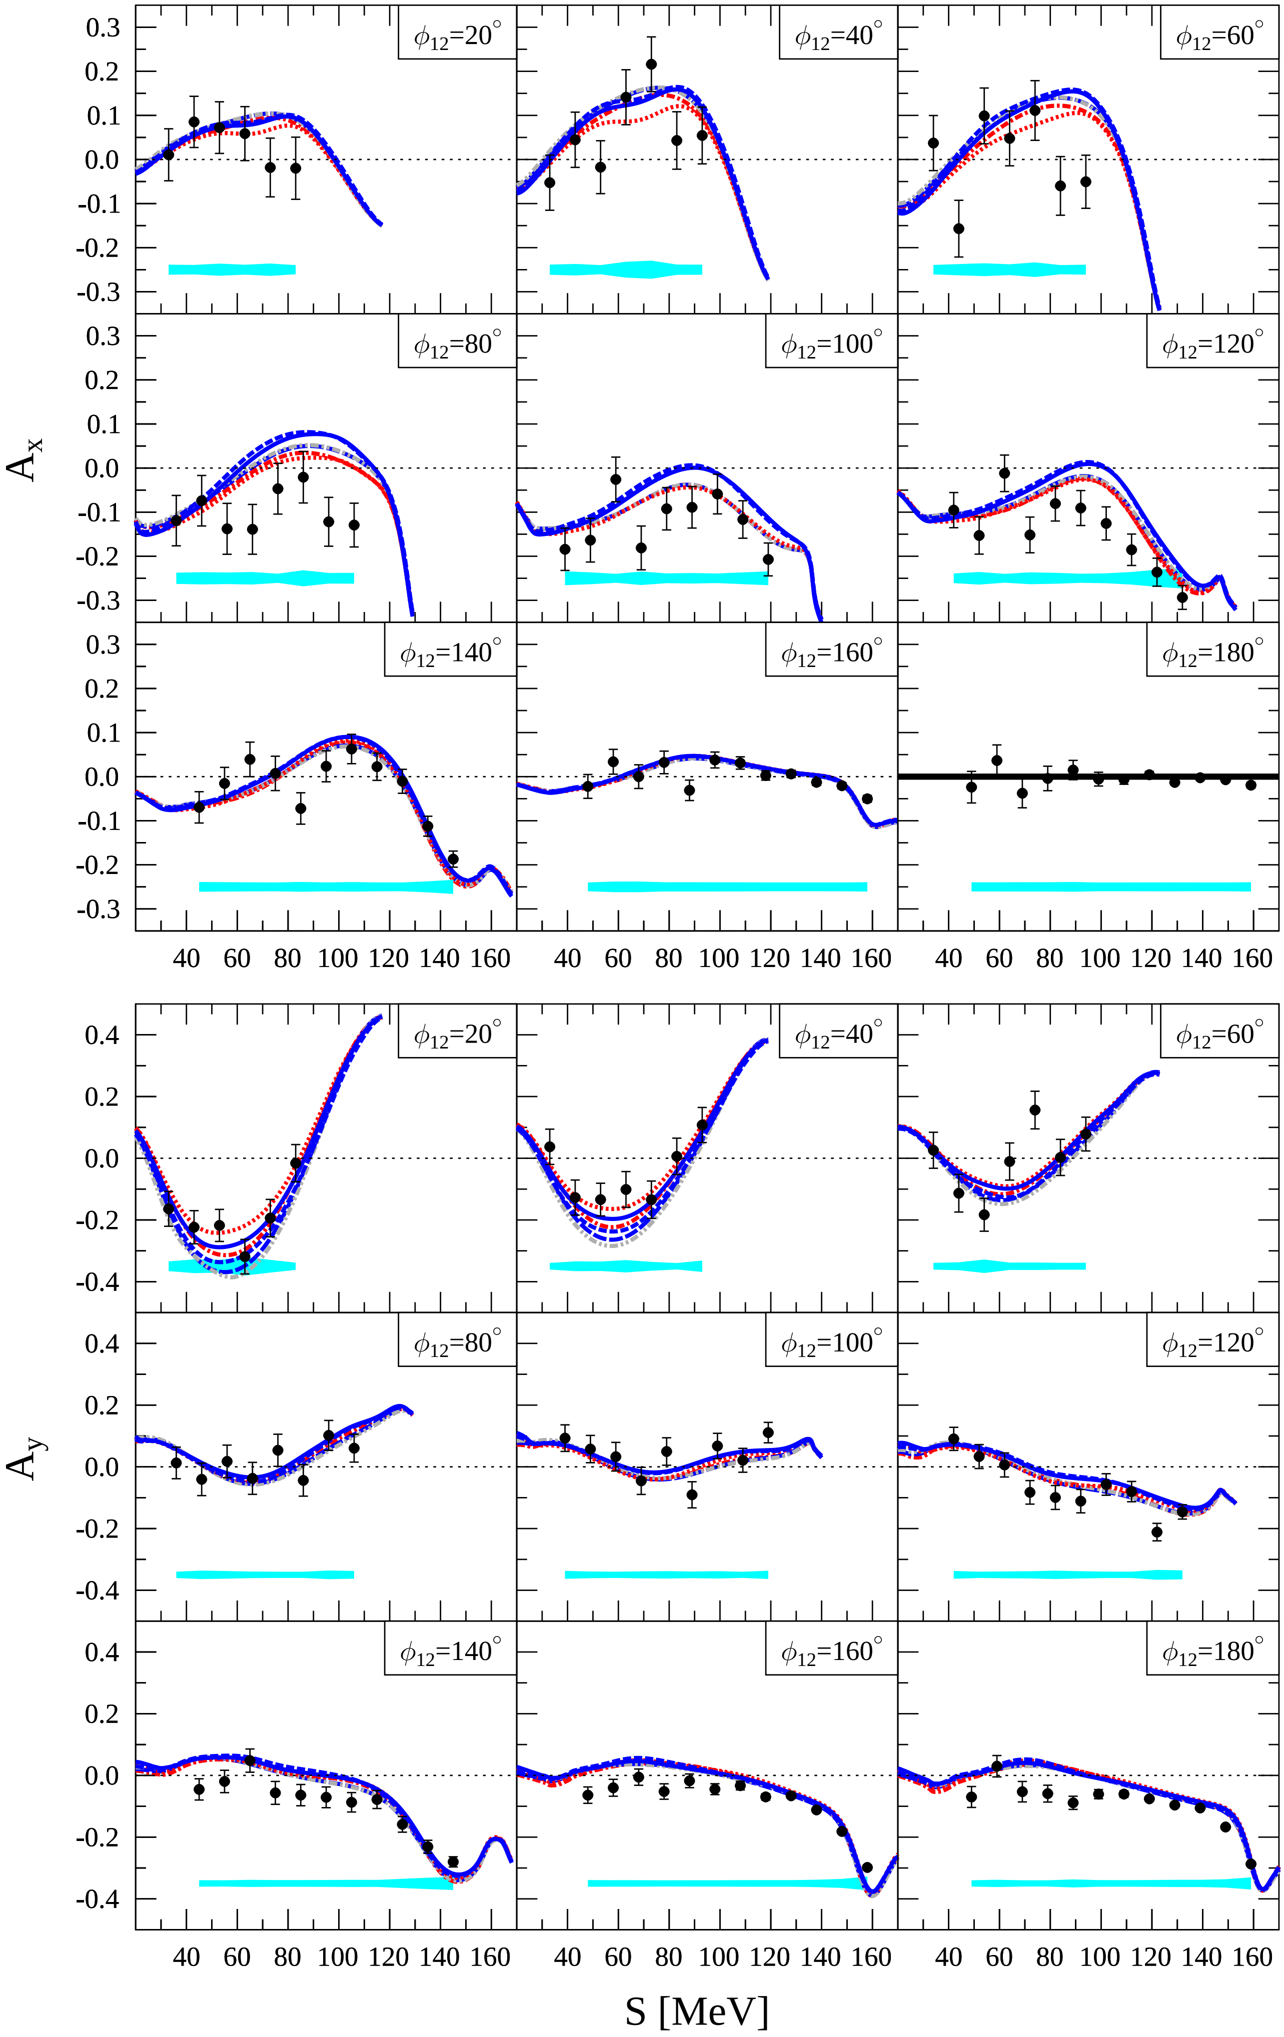


**Fig. 8.** Same as Fig. 1 except for ($\theta_1 = 50°, \theta_2 = 28°$).

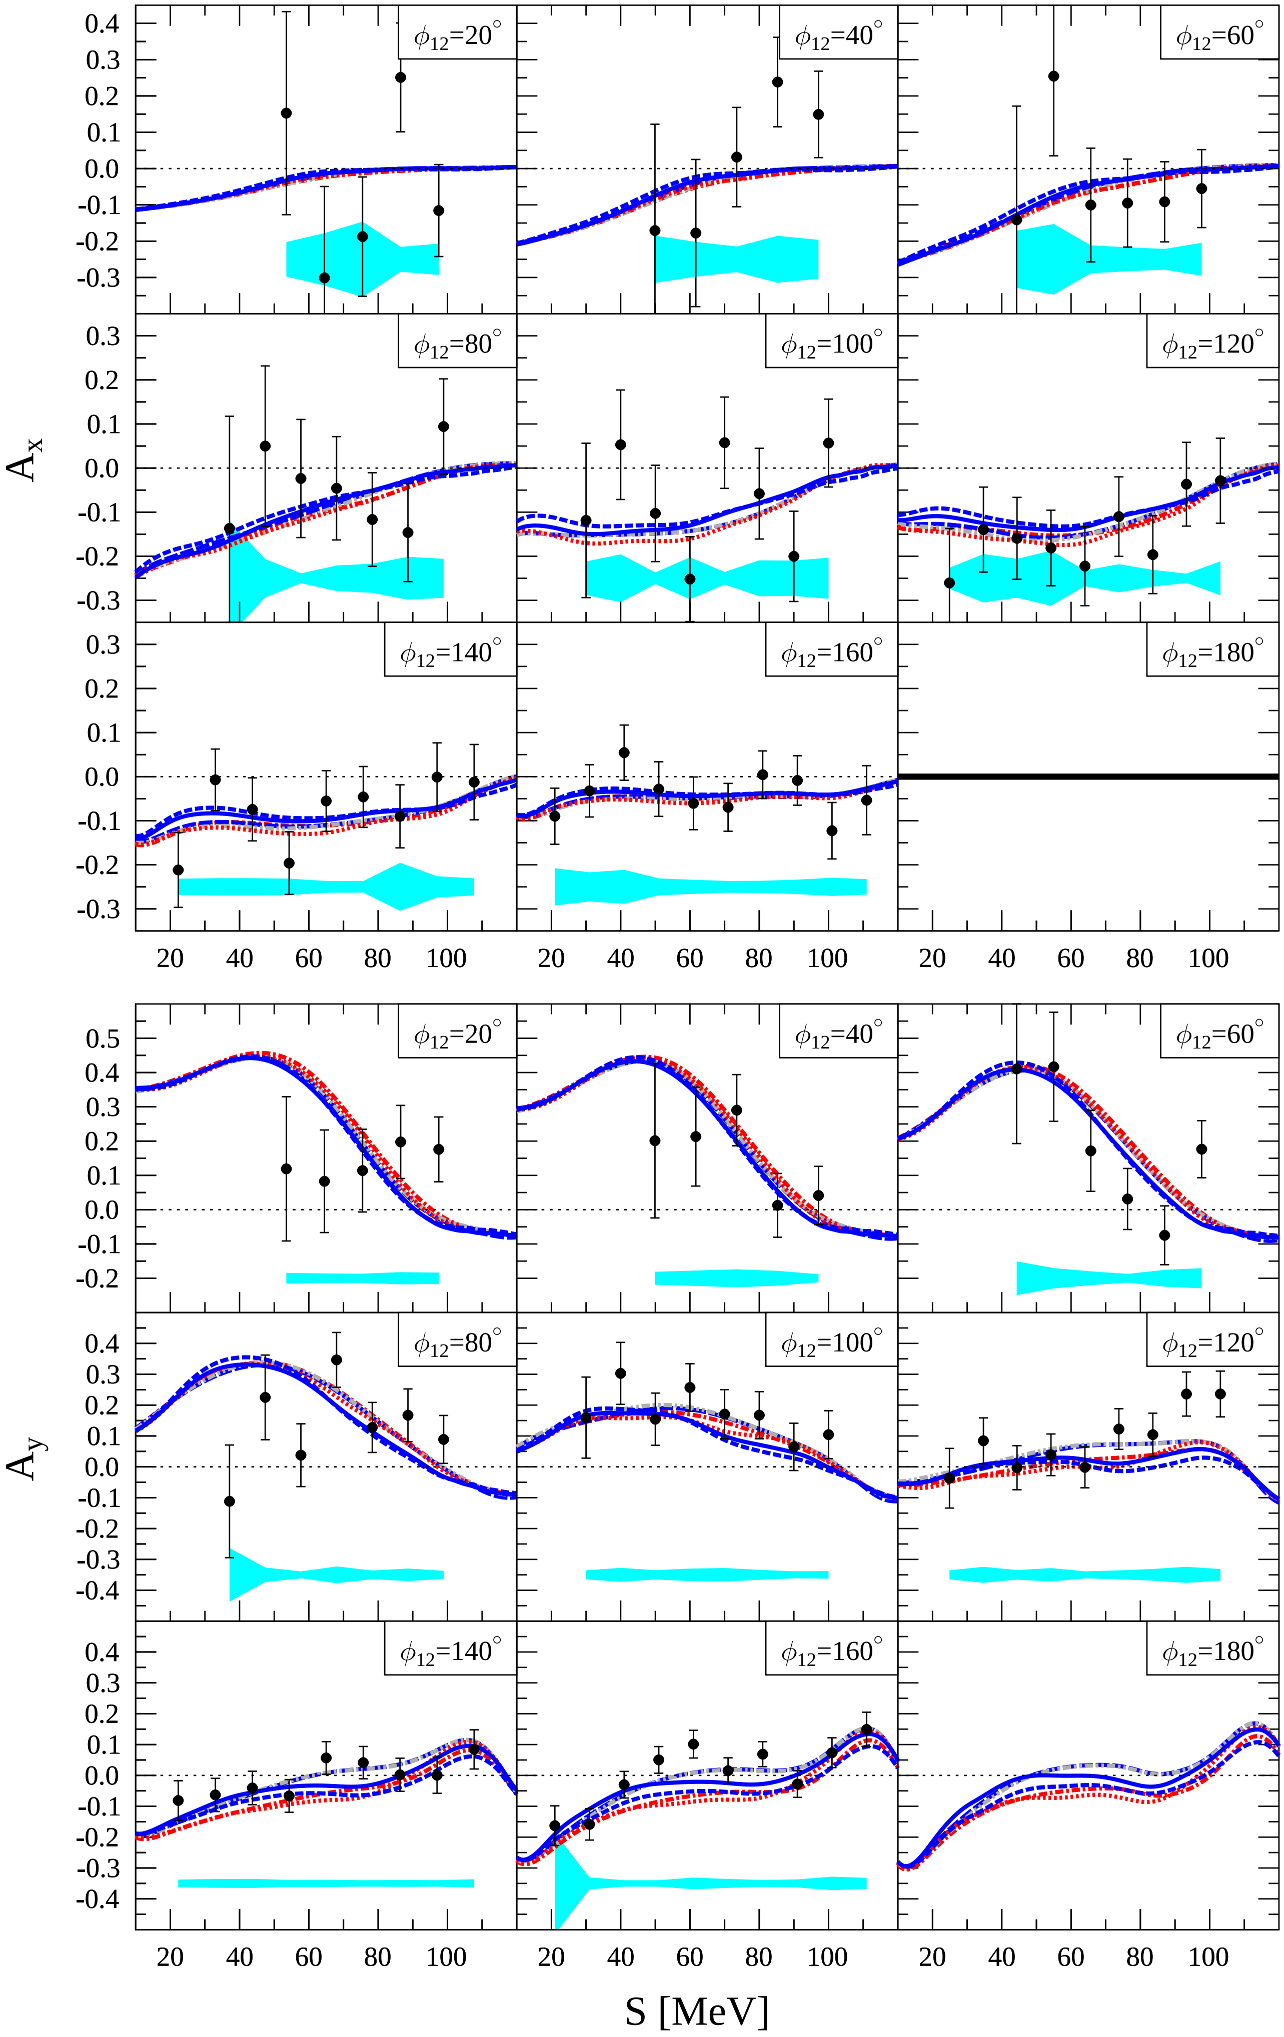


**Fig. 9.** Same as Fig. 1 except for ($\theta_1 = 107^\circ, \theta_2 = 16^\circ$).

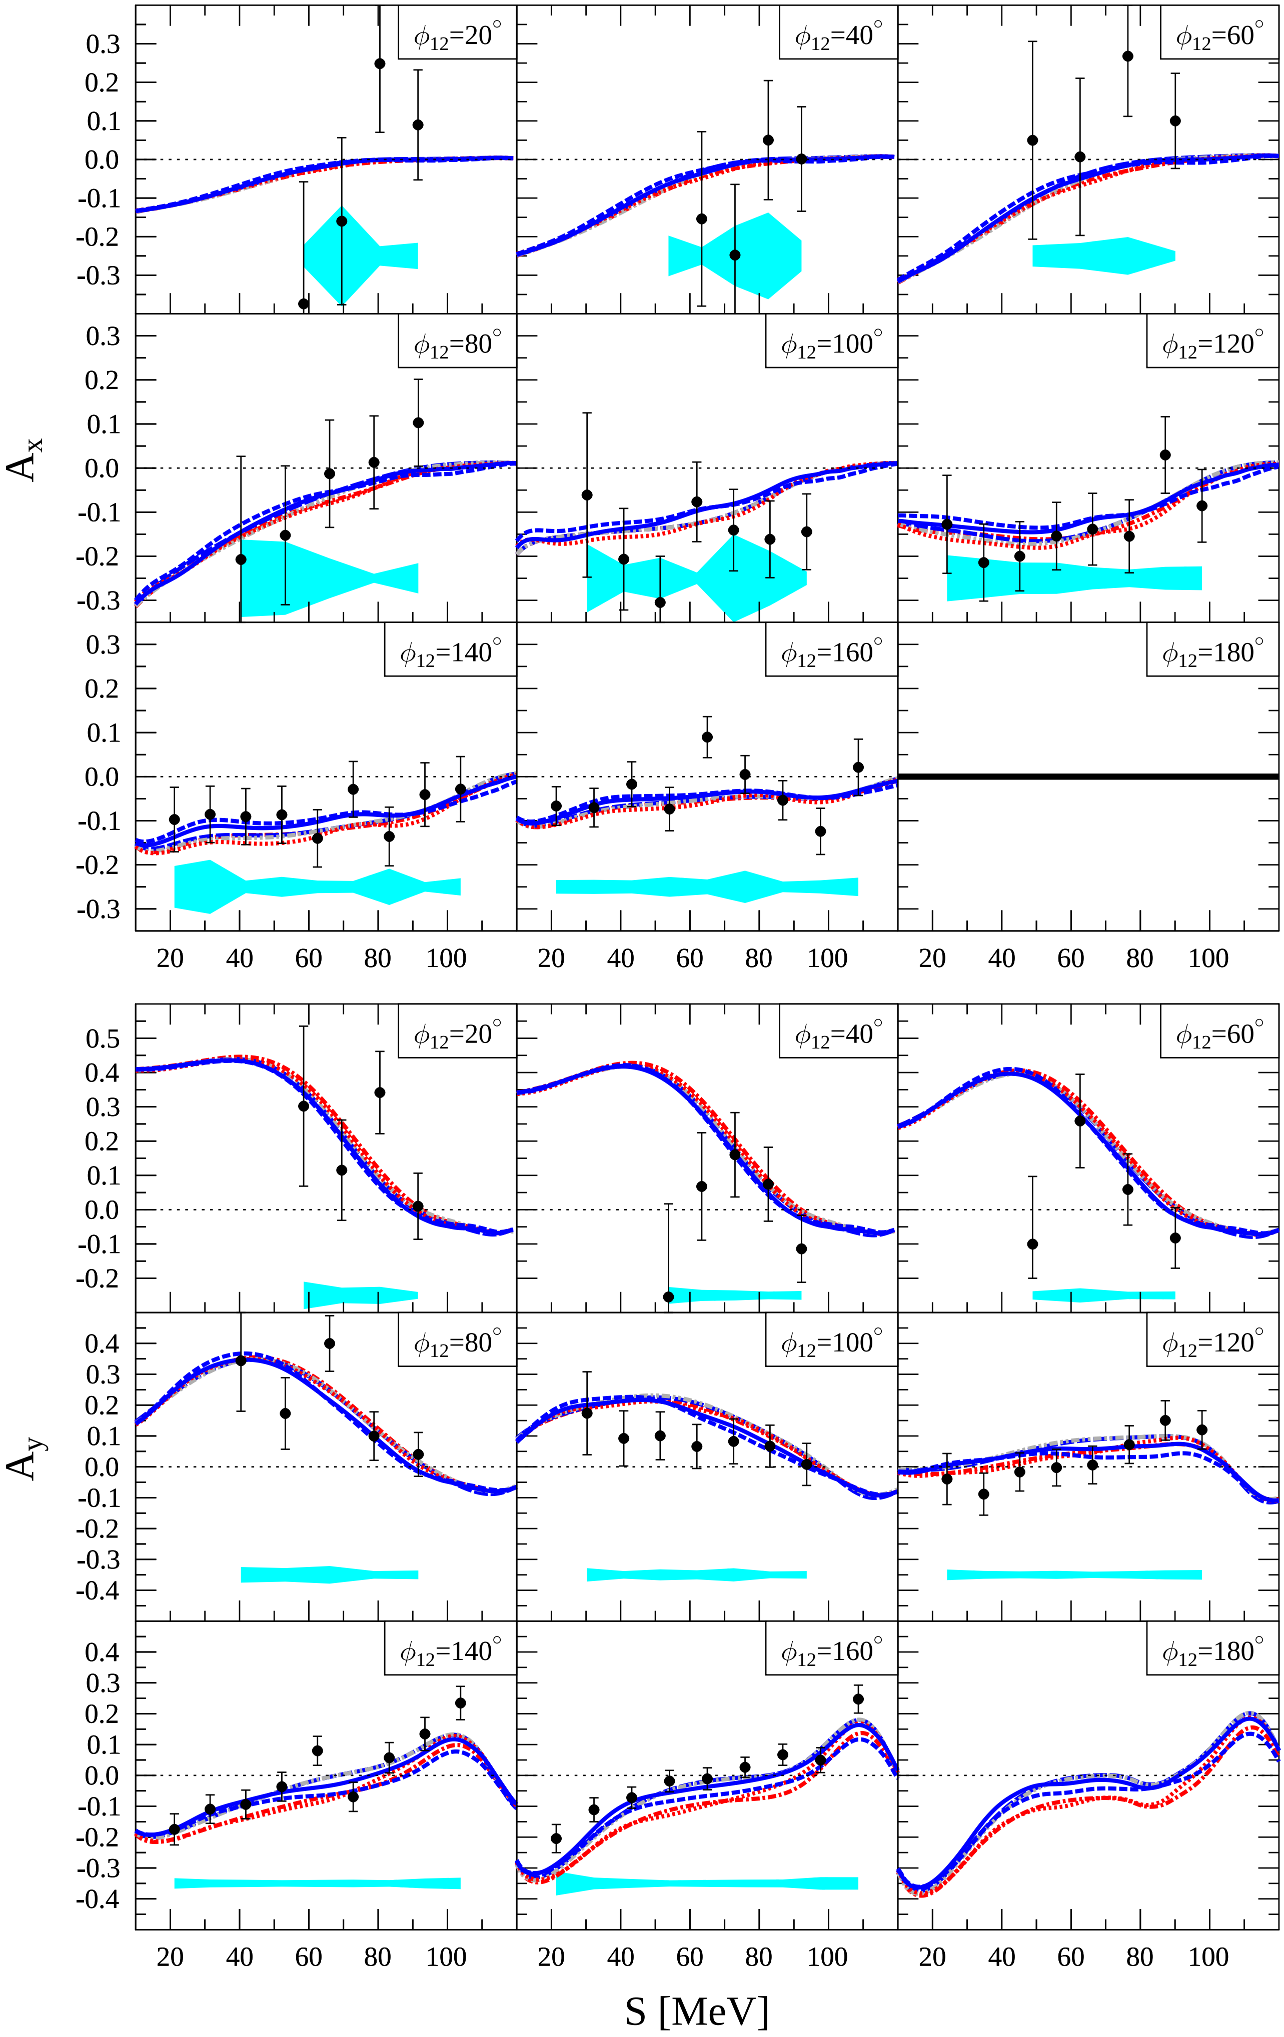


**Fig. 10.** Same as Fig. 1 except for $(\theta_1 = 107^\circ, \theta_2 = 20^\circ)$.

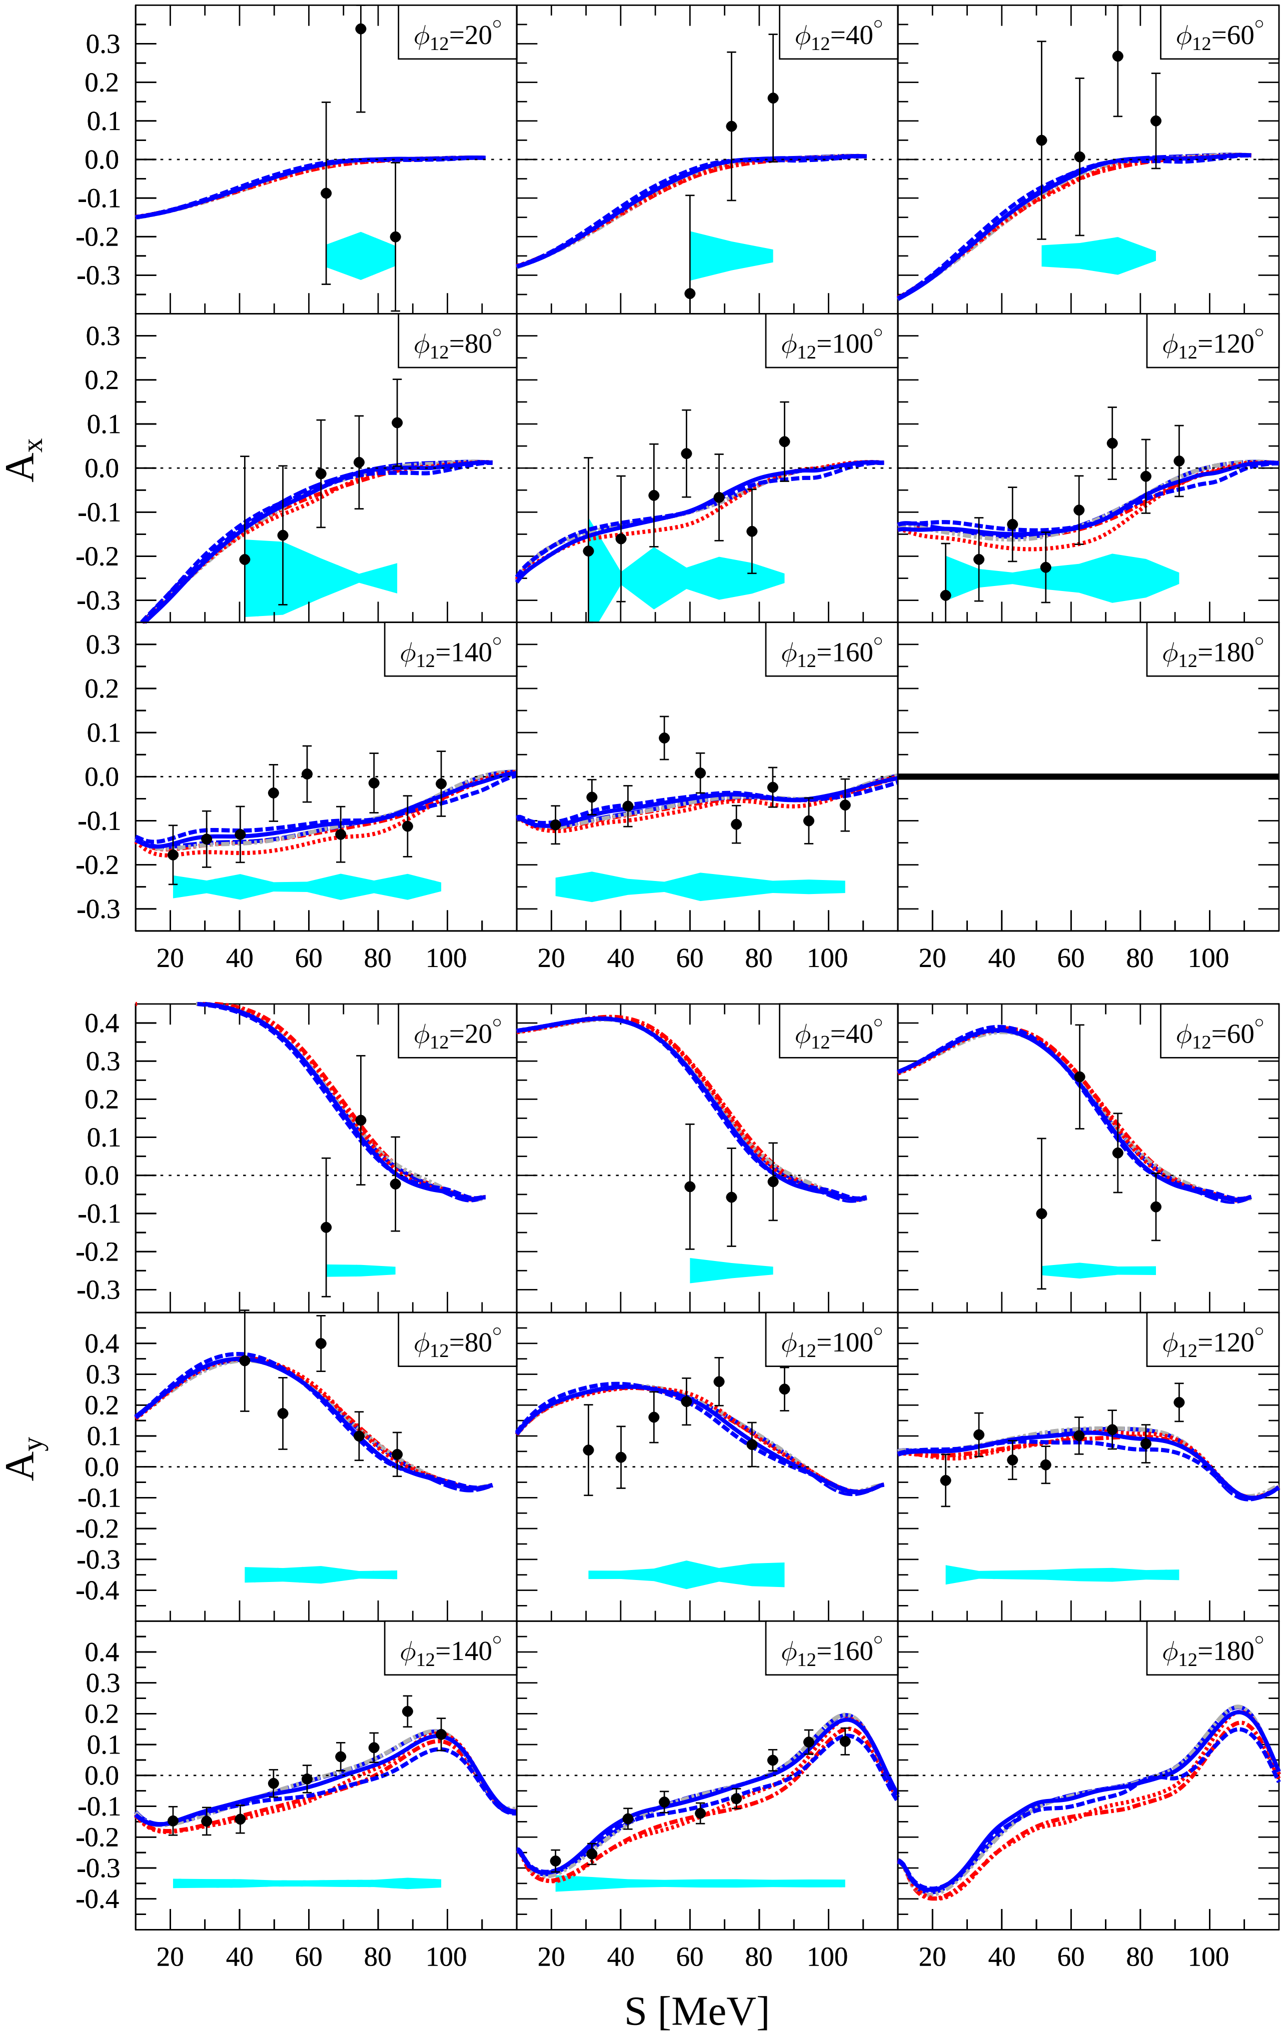


**Fig. 11.** Same as Fig. 1 except for ($\theta_1 = 107°, \theta_2 = 24°$).

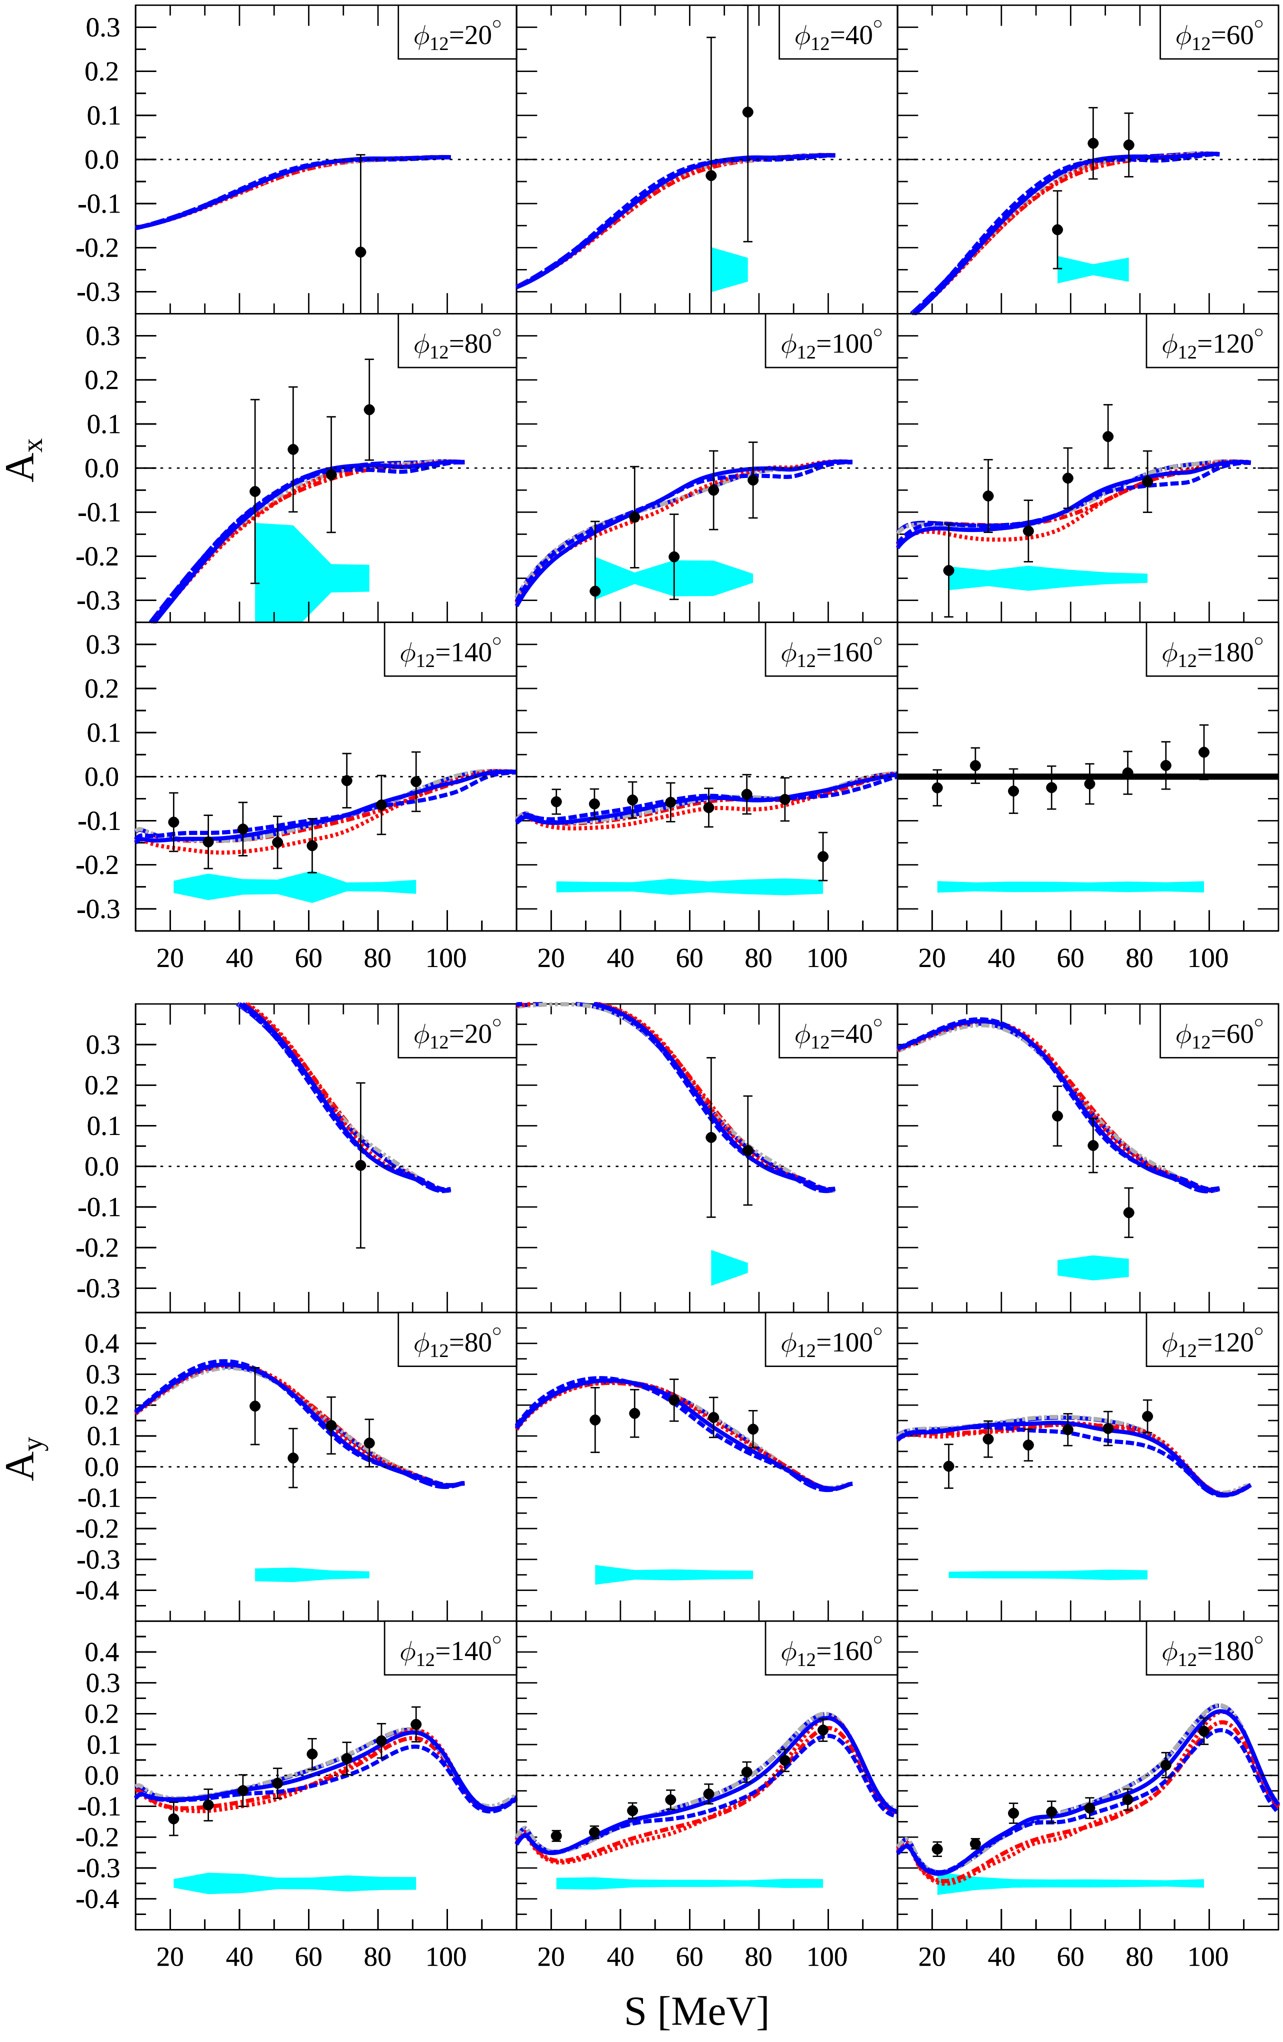


**Fig. 12.** Same as Fig. 1 except for $(\theta_1 = 107^\circ, \theta_2 = 28^\circ)$.

## References

1. R. Machleidt, F. Sammarruca, Y. Song, Phys. Rev. C **53**, R1483 (1996)
2. R. Machleidt, Phys. Rev. C **63**, 024001 (2001)
3. R.B. Wiringa, V.G.J. Stoks, R. Schiavilla, Phys. Rev. C **51**, 38 (1995)
4. H. Witała, W. Glöckle, D. Hüber, J. Golak et al., Phys. Rev. Lett. **81**, 1183 (1998)
5. H. Witała, W. Glöckle, J. Golak, A. Nogga et al., Phys. Rev. C. **63**, 024007 (2001)
6. H. Witała, J. Golak, R. Skibiski, W. Glöckle et al., Nuclear Physics A **827**, 222c (2009)
7. A. Deltuva, Phys. Rev. C **80**, 064002 (2009)
8. A. Deltuva, A. Fonseca, P. Sauer, Phys. Rev. C **72**, 054004 (2005)
9. A. Deltuva, A. Fonseca, P. Sauer, Phys. Rev. C **73**, 057001 (2006)
